# Supplementary material for: LPT++: Efficient Training on Mixture of Long-tailed Experts
Source: arXiv:2409.11323 source file (2024-09-17)
Supplement: Supplementary file 1 [file appendix.tex]

\appendices
\section{Datasets and Evaluation Protocol}\label{supp:datasets}
% Following previous works~\cite{openlongtailrecognition,Kang2020Decoupling}, we evaluate both LPT and LPT++ on two more challenging benchmarks, (\ie, Places-LT and iNaturalist 2018) to demonstrate the effectiveness of our methods. We also report the performance of LPT on CIFAR100-LT to align with previous methods. The details of datasets are shown as follows.
%Following prior works \cite{openlongtailrecognition, Kang2020Decoupling}, we assess the performance of LPT++ on two challenging benchmarks, namely Places-LT and iNaturalist 2018, to validate the efficacy of our methodologies. 
%Additionally, we present the results of out-of-distributed ImageNet~\cite{wang2019learning,imageneta,imagenetr,imagenetv2} to maintain consistency with previous studies. 
%
%Following~\cite{cui2021parametric,tian2021vl,Long2022}, for both Places-LT \cite{zhou2017places} and iNaturalist 2018 \cite{van2018inaturalist}, we stratify the entire dataset based on the number of training images per class into many-shot ($\geq$100 images), medium-shot (20$\sim$100 images), and few-shot ($\leq$20 images) categories. Subsequently, we present the overall accuracy along with accuracy metrics specific to many-shot, medium-shot, and few-shot categories.  
%Similarly, for all out-of-distribution (OOD) ImageNet-variants datasets, we simplify reporting by presenting only the overall accuracy.

In line with previous works \cite{openlongtailrecognition, Kang2020Decoupling}, we evaluate the performance of LPT++ on two challenging benchmarks, Places-LT and iNaturalist 2018, to validate the effectiveness of our approach. Additionally, to ensure consistency with prior studies, we report results on out-of-distribution ImageNet variants~\cite{wang2019learning,imageneta,imagenetr,imagenetv2}.

Following~\cite{cui2021parametric,tian2021vl,Long2022}, we stratify the Places-LT~\cite{zhou2017places} and iNaturalist 2018~\cite{van2018inaturalist} datasets into three categories based on the number of training images per class: many-shot ($\geq$100 images), medium-shot (20–100 images), and few-shot ($\leq$20 images). We then report both the overall accuracy and the accuracy specific to each category. For the out-of-distribution (OOD) ImageNet variants, we simplify our reporting by presenting only the overall accuracy.

\section{Full Implementation Details}\label{app:full_details}
In LPT++, we use the ImageNet-21k pretrained ViT-B/16~\cite{dosovitskiy2021an} as the backbone for  its  visual-only expert, and the CLIP ViT-B/16~\cite{radford2021learning} pretrained model as the backbone for its visual-language expert. The default prompt length is set to 10, with prompts applied across all transformer blocks in the ViT. For group-specific prompts, we fix the number of shared layers at $\text{K} = 6$ and set the prompt size to $\text{m} = 20$, with each prompt also having a length of 10. Although setting $\text{K} = 6$ increases inference costs by 1.5x compared to VPT~\cite{jia2022vpt}—as it involves using ViT with a shared prompt to generate the output class token as a query, followed by reusing features from the 6-th block and performing inference with both shared and group prompts for the last 6 blocks—this approach achieves higher accuracy and is more efficient than performing inference twice, as done in methods such as \cite{wang2022learning}. During both training and testing, we use prompt ensembles with $k = 2$. For visual adapter~\cite{chen2022adaptformer}, the hidden dimension is set to 8 for Place-LT and 256 for iNaturalist 2018 to accommodate the varying number of classes. The total number of additional parameters (excluding linear classifiers for simplicity) is 1.19 million, and both prompts are initialized using a truncated normal distribution.

During training in both Phase 1 and Phase 2, we use the SGD optimizer with a momentum of 0.9 to optimize the shared and group-specific prompts. A weight decay rate of 1e-2 is applied to ensure a stable training process for LPT++. We employ a cosine learning rate scheduler with an initial learning rate of $0.002 \times \frac{B}{256}$ and 5 warmup epochs, where $B$ denotes the batch size. For datasets like Places-LT, CIFAR100-LT, and ImageNet-LT, both Phase 1 and Phase 2 of LPT++ are trained for $\text{E} = 40$ epochs each; for iNaturalist 2018, due to its larger training dataset, both phases are optimized for $\text{E} = 80$ epochs each. In the asymmetric GCL loss, we set $\lambda_{+} = 0$ and $\lambda_{-} = 4$. For Phase 2, the initialized weight $\gamma$ used in ${\mathbf{I}}_{\text{ins}}$ is set to 0.5. All training and testing images are resized to $224 \times 224$. 
And for phase 3, we optimize the MoE scorer for 50 epochs with the learning rate of 0.01. 
Data augmentation during both training phases of LPT++ includes random cropping, resizing operations, and the Mixup technique. All experiments are implemented using PyTorch~\cite{NEURIPS2019_9015} and conducted on a single RTX A6000 GPU.

\begin{table*}[h]
   \centering
   \begin{minipage}[t]{0.48\textwidth}

      \centering
      \caption{Ablation Study of different pretrained models. Both more pretraining data and better pretraining algorithms benefit to LPT.}
      % \vspace{-1em}
      \setlength{\tabcolsep}{9.6pt} % column spacing
	%  row spacing
	  		{ \fontsize{8.3}{3}\selectfont{
      \begin{tabular}{l|c|cc}
         \toprule
         \bf Method & \bf Data & \bf Phase 1 & \bf LPT \\
         \midrule
         DINO & IN1k &40.65 &42.18 \\
         Mugs & IN1k &41.92 &43.66 \\
         Supervised & IN1k & 41.33 & 42.71 \\
         Supervised & IN21k & \textbf{49.41} & \textbf{50.50} \\
         \bottomrule
      \end{tabular}}}
      \label{table:ablation_pretrain}
   \end{minipage}\hspace{4mm}
   \begin{minipage}[t]{0.48\textwidth}

      \centering
      \caption{Ablation Study of the size of group-specific prompts. Prompt set with 20 individual group prompts performs better. }
      % \vspace{-1em}
      \setlength{\tabcolsep}{8.6pt} % column spacing
	%  row spacing
	  		{ \fontsize{8.3}{3}\selectfont{
      \begin{tabular}{l|c|c}
         \toprule
         \textbf{Group Size} & \textbf{Parameters}  & \textbf{Phase 2 Acc} \\
         \midrule
         5 & 0.23M & 49.81 \\
         10 & 0.46M & 49.90 \\
         20 & 0.92M & \textbf{50.50} \\
         40 & 1.84M & 49.87 \\
         \bottomrule
      \end{tabular}}}
      \label{table:ablation_setsize}
   \end{minipage}
   % \vspace{-1em}
   \end{table*}

\begin{figure}[tp]
   \centering
   \begin{minipage}{0.46\textwidth}
      \centering
            
      \includegraphics[width=\textwidth]{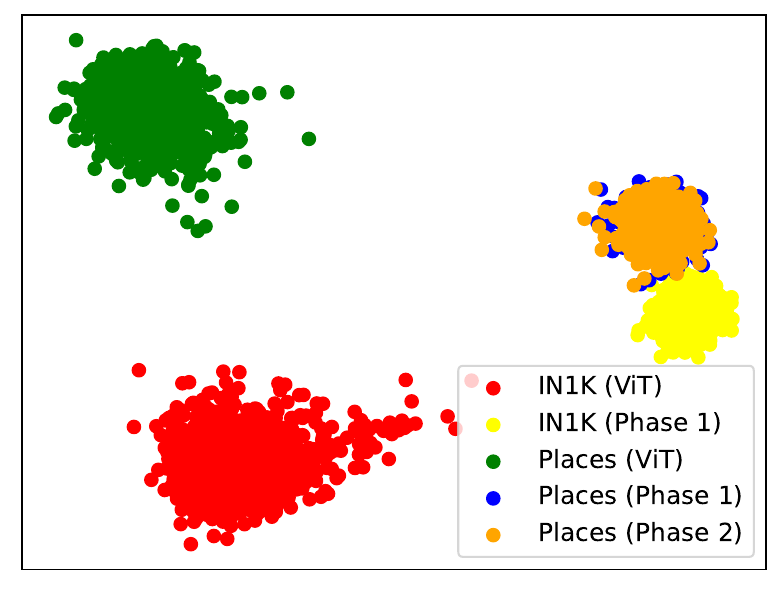}
      % \vspace{-2em}
      \caption{LDA visualization of LPT++.%\vspace{-0.6em} 
      } 
      \label{fig:ablation_domain_shift}
   \end{minipage}
% \hspace{-1mm}
   \begin{minipage}{0.46\textwidth}

      \centering
      \captionsetup{type=table}
      \caption{Quantitative analysis of features learned by Phase 1 of LPT++(V) and Phase 2 of LPT++(V). Features from phase 2 of LPT++(V) obtains the similar $\gamma$ value while obtaining larger inter-class distance. }
      % \vspace{0.5em
    		\setlength{\tabcolsep}{4.6pt} % column spacing
  %  row spacing}
      	  		{ \fontsize{8.3}{3}\selectfont{
      \begin{tabular}{l|cc}
         \toprule
         \textbf{Method} & {Phase 1}  & {Phase 2} \\
         \midrule
        %  \bf Pretrain Data & IN21k & IN21k \\
        %  \hline
        %  \bf Fine-tuned & - & \checkmark \\
        %  \hline
         \bf Inter-class distance & 15.8 & \textbf{16.1} \\
         \bf Inner-class / inter-class $\gamma$ & \textbf{0.237} & {0.242} \\
         % \hline
        %  \bf K-NN Acc & {30.80\%} & \textbf{31.90\%} \\
         \bottomrule
      \end{tabular}}}
      \label{table:ablation_discriminative}
   \end{minipage}
%   \vspace{-1.5em}
\end{figure}

\begin{table*}[h]
\centering
\begin{minipage}[t]{0.48\textwidth}

   \centering
   \caption{Ablation Study of Decoupled or Joint Training. Decoupled Training is better. }
   % \vspace{-0.5em}
   \setlength{\tabcolsep}{12.6pt} % column spacing
	%  row spacing
	  		{ \fontsize{8.3}{3}\selectfont{
   \begin{tabular}{l|cc}
      \toprule
      \bf Method & \bf Epochs & \bf Overall \\
      \midrule
      Joint 1\&2 & 80 & 47.48  \\
      Decoupled 1\&2 & 40+40 & \textbf{50.50} \\
      \bottomrule
   \end{tabular}}}
   \label{table:ablation_decoupled}
\end{minipage}\hspace{4mm}
\begin{minipage}[t]{0.48\textwidth}

   \centering
   \caption{Ablation study of query function in phase 2. Using phase 1 as query is better. }
   % \vspace{-0.5em}
   \setlength{\tabcolsep}{10.6pt} % column spacing
	%  row spacing
	  		{ \fontsize{8.3}{3}\selectfont{
   \begin{tabular}{l|cc}
      \toprule
      \textbf{Query Func} & \textbf{K-NN Acc}  & \textbf{Phase 2 Acc} \\
      \midrule
      ViT-B & 32.11 & 49.81 \\
      Phase 1 & \textbf{36.16} & \textbf{50.50} \\
      \bottomrule
   \end{tabular}}}
   \label{table:ablation_query}
\end{minipage}
% \vspace{-1em}
\end{table*}

\section{More Analysis}
% \zp{maybe here you should use LPT++ instead of LPT, since the whole paper focus on LPT++. If you do not want to change, please explain why using LPT for analysis instead of LPT++.}
Finally, to comprehensively analyze the other modules in LPT++, we focus on LPT++(V) and explore the effect from pretrained models and different hyper-parameters. %More analysis will be shown in Appendix. 

\subsection{The Effect of Shared Prompt and Group Prompts. }\label{sec:ablation_different_prompts_more}
To further explore the impact of shared and group prompts, we conduct additional quantitative and qualitative analyses on the Places-LT dataset, building upon the ablation study discussed in Section \ref{sec:ablation}. As detailed in Section \ref{sec:method}, shared prompts are designed to capture domain-specific knowledge from the training data, while group prompts aim to enhance the extraction of group-specific features from corresponding clusters. To validate this hypothesis, we applied Linear Discriminant Analysis (LDA) to analyze features extracted from LPT++(V) (Phase 1), LPT++(V) (Phase 2), and features obtained directly from the pretrained ViT without any prompts. The visualization results, depicted in Figure \ref{fig:ablation_domain_shift}, reveal significant overlap in the distributions of features from LPT++(V) (Phase 1) and LPT++(V) (Phase 2), confirming that shared prompts in Phase 1 effectively capture domain-specific knowledge.

Moreover, we  also analyze  the  value of $\gamma$ and inter-class distances of features from LPT++(V) (Phase 1) and LPT++(V) (Phase 2), summarized in Table \ref{table:ablation_discriminative}, shows that both phases exhibit similar   values of $\gamma$. However, LPT++(V) (Phase 2) demonstrates a larger inter-class distance, indicating that group prompts contribute to enhancing class discriminative capabilities.

\subsection{Different Model Size and Pretrained Models. }
Here we assess the compatibility of LPT++ by evaluating its performance using ViT-Tiny, ViT-Small, and ViT-Base models pretrained on ImageNet-21k \cite{deng2009imagenet}. 
To eliminate the effect from other components, we conduct ablation study on LPT++(V) single model. 
The results, presented in Table \ref{table:ablation_scale}, indicate that LPT++ achieves accuracies of 37.40\%, 44.66\%, and 50.50\% with ViT-Tiny, ViT-Small, and ViT-Base, respectively. These results surpass models equipped solely with shared prompts by 4.85\%, 4.16\%, and 1.09\%, respectively, underscoring LPT++'s compatibility across different ViT scales. Notably, ViT-Tiny and ViT-Small, despite having fewer parameters compared to ViT-Base, benefit significantly from the integration of shared and group-specific prompts, leading to substantial improvements in accuracy.

We also retain the ViT-B model to assess the impact of LPT++ across various pretrained models \cite{pmlr-v139-touvron21a,caron2021emerging,zhou2022mugs,dosovitskiy2021an}. The evaluation results demonstrate that superior self-supervised learning methods and increased pretraining data correlate with higher accuracy, reaching 50.50\% with LPT++(V). Further details are provided in Sec. \ref{sec:pretrained_models}.

\subsection{Decoupled Training. }
%To investigate the impact of decoupled training, we conducted an ablation study where we separately optimized the shared prompt and group-specific prompts. To ensure fairness, we trained the joint model for 80 epochs. The results are presented in Table \ref{table:ablation_decoupled}, showing that LPT achieved 50.07\% overall accuracy with decoupled training, surpassing joint training by 2.59\%. These findings suggest that during joint training, simultaneous updates to the shared prompt compromise the optimization of the query function, leading to inferior matching results. In contrast, decoupled training maintains a fixed yet optimal shared prompt as the query function, thereby achieving superior results.

To investigate the impact of decoupled training, we conducted an ablation study in which we separately optimized the shared and group-specific prompts. For fairness, we train the joint model for 80 epochs. As shown in Table \ref{table:ablation_decoupled}, LPT++(V) achieved 50.50\% overall accuracy with decoupled training, surpassing joint training by 2.59\%. These findings suggest that during joint training, simultaneous updates to the shared prompt compromise the optimization of the query function, leading to suboptimal results. In contrast, decoupled training maintains a fixed yet optimal shared prompt as the query function, resulting in superior outcomes.

\subsection{Query Function and Group Size $\text{m}$. }
%We conducted further analysis on the query function and group size $\text{m}$. In \cite{wang2022learning}, a pretrained ViT was used as the query function. To determine whether using Phase 1 of LPT as the query function yields better results, we conducted an ablation study on the query function. Specifically, following the LPT design, we employed cosine similarity as the distance metric and evaluated the K-NN accuracy of two query functions. The results are summarized in Table \ref{table:ablation_query}. Phase 1 achieved 36.16\% K-NN accuracy, surpassing pretrained ViT-B by 4.05\%, indicating that queries from Phase 1 provide higher-quality matches for prompts. Moreover, compared to using ViT-B as the query function, using Phase 1 achieved an overall accuracy of 50.07\%, further demonstrating the effectiveness of Phase 1 as a query function. Additionally, we varied the size of $\mathcal{R}$, denoted as $\text{m}$, from 5 to 40, finding that LPT exhibits robustness across different $\text{m}$ values, achieving its best accuracy of 50.07\% when $\text{m}=20$.

We further analyzed the query function and group size ($m$). In \cite{wang2022learning}, a pretrained ViT was used as the query function. To determine whether using Phase 1 of LPT++(V) as the query function yields better results, we conducted an ablation study. Specifically, following the LPT++(V) design, we used cosine similarity as the distance metric and evaluated the K-NN accuracy of two query functions. The results, summarized in Table \ref{table:ablation_query}, show that Phase 1 achieved 36.16\% K-NN accuracy, surpassing pretrained ViT-B by 4.05\%, indicating that queries from Phase 1 provide higher-quality matches for prompts. Additionally, using Phase 1 as the query function achieved an overall accuracy of 50.50\%, further demonstrating its effectiveness. We also varied the group size ($m$) from 5 to 40, finding that LPT++(V) is robust across different values of $m$, achieving its best accuracy of 50.50\% when $m=20$

\begin{table}
   \centering
   \caption{Ablation Study of the number of blocks with only shared blocks, \textit{i.e.}, $\text{K}$. Quantitative results show that $\text{K}=6$ performs better for phase 2 of LPT. }
   % \vspace{-1em}
   \setlength{\tabcolsep}{13.6pt} % column spacing
	%  row spacing
	  		{ \fontsize{8.3}{3}\selectfont{
   \begin{tabular}{l|c|c|c}
      \toprule
      \textbf{$\text{K}$} & 8  & 6 & 4 \\
      \midrule
      \textbf{Param Num} & 0.61M & 0.92M & 1.23M \\
      \textbf{Overall Acc} & 49.77 & \textbf{50.50} & 49.92 \\
      \bottomrule
   \end{tabular}}}
   \label{table:ablation_k}
% \vspace{-1em}
\end{table}

\begin{table}
   \centering
   \caption{Ablation Study of ensemble prompt number ${k}$ in LPT++. We report the results on LPT++(V) to clearly show the effect from $k$. Quantitative results show that ${k}=2$ and $3$ achieve better results, thus we select $t=2$ in LPT++. }
   % \vspace{-1em}
   \setlength{\tabcolsep}{7.6pt} % column spacing
	%  row spacing
	  		{ \fontsize{8.3}{3}\selectfont{
   \begin{tabular}{l|c|c|c|c}
      \toprule
      \textbf{Ensemble Num ${k}$} & 1  & 2 & 3 & 4 \\
      \midrule
      \textbf{Overall Acc} & 49.93 & \textbf{50.50} & 50.00 & 49.93 \\
      \textbf{Few-shot Acc} & 46.32 & \textbf{49.40} & 46.87 & 46.84 \\
      \bottomrule
   \end{tabular}}}
   \label{table:ablation_t}
% \vspace{-1em}
\end{table}

\subsection{Pretrained Models}\label{sec:pretrained_models}
% We also evaluate our LPT on various pretrained models from different pretraining algorithms and different pretraining data scale. Specifically, we keep using ViT-B/16 structure and select DeiT~\cite{pmlr-v139-touvron21a}, DINO~\cite{caron2021emerging} and Mugs~\cite{zhou2022mugs} pretrained on ImageNet-1k~\cite{deng2009imagenet}, meanwhile using ViT-B~\cite{dosovitskiy2021an} pretrained on ImageNet-21k as baseline model. Evaluation results are shown as Table~\ref{table:ablation_pretrain}. With the same ImageNet-1k pretraining data, LPT with Mugs achieves 41.92\% accuracy after phase 1 and 43.66\% accuracy after phase 2, which surpasses other two pretrained models. Meanwhile, VPT with ImageNet-21k pretrained model achieves 50.07\% accuracy and largely surpasses LPT with DeiT-B. These results indicate that pretrained models from better algorithms or larger pretraining data lead to better efficient tuning results with long-tailed target data.
We also evaluate our LPT++(V) using various pretrained models sourced from different pretraining algorithms and datasets of varying scales. Specifically, we utilized the ViT-B/16 architecture, employing pretrained models such as DeiT~\cite{pmlr-v139-touvron21a}, DINO~\cite{caron2021emerging}, and Mugs~\cite{zhou2022mugs} trained on ImageNet-1k~\cite{deng2009imagenet}. In addition, we used ViT-B~\cite{dosovitskiy2021an} pretrained on ImageNet-21k as our baseline model. The evaluation outcomes are presented in Table~\ref{table:ablation_pretrain}. 
When trained with the same ImageNet-1k data, LPT++(V) using the Mugs model achieved an accuracy of 41.92\% after phase 1 and 43.66\% after phase 2, outperforming the other two pretrained models. Meanwhile, utilizing the ViT-B model pretrained on ImageNet-21k resulted in an accuracy of 50.50\%, significantly surpassing LPT++(V) with DeiT-B. These findings underscore that pretrained models derived from superior algorithms or larger pretraining datasets yield enhanced performance when fine-tuned with long-tailed target data.

\subsection{Size of Group-Specific Prompts}\label{sec:ablation_setsize}
% We also conduct ablation study about the size of group-specific prompts. Generally, we start each phase 2 training from the same phase 1 model, and only change the group size of the group-specific prompts. The corresponding evaluation results are shown as Table~\ref{table:ablation_setsize}. When the size of group-specific prompts increasing to 20, the accuracy of LPT increases from 49.81\% to 50.07\%. However, when we further increase the size to 40, the final accuracy declines to 49.87\%. A possible reason is that, some classes in the dataset may share some similar group-specific feature or knowledge, such that features from instances in corresponding classes may be similar. Thus instances from these classes can be seen as a cluster and can be matched into the same prompt. Since the number of different attributes is limited, we only need a fixed number (\textit{e.g.}, 20) of group prompts to handle the whole dataset and achieve better accuracy. Besides, using too many group prompts may increase the difficulty of clustering and optimization, which affects the final accuracy. 

We also conducted an ablation study on the size of group-specific prompts. Typically, each phase 2 training session commences with the same phase 1 model, with the sole modification being the group size of the group-specific prompts. The corresponding evaluation outcomes are detailed in Table~\ref{table:ablation_setsize}. Increasing the size of group-specific prompts to 20 resulted in an accuracy improvement for LPT++(V) from 49.81\% to 50.50\%. However, further increasing the size to 40 led to a decrease in final accuracy to 49.87\%. 
This variation may be attributed to some classes within the dataset sharing similar group-specific features or knowledge, thereby allowing instances from these classes to be clustered together under the same prompt. Given the finite number of distinct attributes, a fixed number (\emph{e.g.}, 20) of group prompts suffices to effectively manage the entire dataset and achieve superior accuracy. Moreover, employing an excessive number of group prompts can complicate clustering and optimization processes, thereby adversely affecting final accuracy.

\begin{table}

   \centering
   \caption{
   Ablation Study of dual sampling in phase 2. Adding dual sampling strategy with proper small $\gamma$ (\textit{e.g.}, 0.5).
   }
   % \vspace{-1em}
   \setlength{\tabcolsep}{6.6pt} % column spacing
	%  row spacing
	  		{ \fontsize{8.3}{3}\selectfont{
   \begin{tabular}{l|cc|cc}
      \toprule
      \textbf{Method} & \textbf{Dual} & \textbf{$\gamma$} & \textbf{Overall} & \textbf{Many-shot} \\
      \midrule
      (a) balanced sampling & - & - & 49.90 & 47.67 \\
      (b) dual w/ small $\gamma$ & \checkmark & 0.5 & \textbf{50.50} & 47.80 \\
      (c) dual w/ large $\gamma$ & \checkmark & 1.0 & 49.62 & \textbf{50.06} \\
      \bottomrule
   \end{tabular}}}
   \label{table:ablation_dual_sampling}
% \vspace{-1em}
\end{table}

\begin{table}

   \centering
   \caption{Ablation Study of asymmetric GCL Loss on LPT++(V). Introducing gradient re-weighting into GCL Loss can further improve overall accuracy in long-tailed classification. }
   % \vspace{-1em}
   \setlength{\tabcolsep}{7.6pt} % column spacing
	%  row spacing
	  		{ \fontsize{8.3}{3}\selectfont{
   \begin{tabular}{l|cccc}
      \toprule
      \textbf{Loss Function} & \textbf{Overall}  & \textbf{Many} & \textbf{Medium} & \textbf{Few} \\
      \midrule
      GCL~\cite{Li2022Long} & 49.58 & 48.19 & 52.62 & 45.75 \\
      $\mathcal{L}_{\text{A-GCL}}$ & 50.50 & 47.80 & 53.20 & 49.40 \\
      \bottomrule
   \end{tabular}}}
   \label{table:asym_gcl}
% \vspace{-1em}
\end{table}

\subsection{Effect of K}\label{sec:ablatioin_k}
% Next we further analyze the effect of $\text{K}$, which stands for the number of blocks with only the shared prompt $\mathbf{u}$. Intuitively, the less $K$ means more parameters are inserted into more transformer blocks to conduct group prompts tuning and should lead to better performance. To verify this hypothesis, we set $\text{K}=4/6/8$ and conduct corresponding ablation study. Evaluation results are shown in Table~\ref{table:ablation_k}. LPT with $\text{K}=6$ achieves the best performance and surpasses LPT with $\text{K}=8$ by 0.3\% in terms of overall accuracy. Meanwhile, LPT with $\text{K}=4$ achieves similar performance with $\text{K}=6$ counterpart, but does not lead to significant performance improvement with more parameters. The possible reason is that: \textbf{1)} too large $\text{K}$ could restrict the group-specific knowledge gathering ability of group-specific prompts, since only a few layers are utilized to extract group-specific features from long-tailed data; and \textbf{2)} compared to $K=4$, LPT with $\text{K}=6$ fully leverages the adapted feature representation from phase 1, thus reducing the difficulty of optimization and achieving better accuracy. Therefore, we choose $\text{K}=6$ for final LPT during experiments.
Next, we proceed to analyze the impact of $K$, denoting the number of blocks exclusively utilizing the shared prompt $\mathbf{u}$. Intuitively, reducing $K$ implies more parameters are allocated across additional transformer blocks for group prompt refinement, potentially enhancing performance. To substantiate this hypothesis, we set $K = 4/6/8$ and conducted the corresponding ablation study. The evaluation results are presented in Table~\ref{table:ablation_k}. 
Among these configurations, LPT++(V) achieves optimal performance with $K = 6$, surpassing the accuracy of other candidates by 0.7\%. 
% Meanwhile, LPT++(V) with $K = 4$ achieves comparable performance to $K = 6$ but does not exhibit significant performance gains despite increased parameter usage. 
%
This outcome can be explained by two factors: (1) A larger $K$ may constrain the ability of group-specific prompts to gather specialized knowledge from long-tailed data, as fewer layers are dedicated to extracting these features. (2) Compared to $K = 4$, employing $K = 6$ fully leverages the adapted representations from phase 1, thereby reducing optimization challenges and improving accuracy.
%
% Based on these findings, we select $K = 6$ for the final LPT configuration in our experiments.

\subsection{Effect of Ensemble Number \textit{k}}\label{sec:ablation_t}
% We also analyze the effect of ensemble token number ${k}$ in phase 2. Intuitively, introducing can lead to better accuracy for tail classes since more class-specific knowledge are utilized for recognition. Therefore we set ${k}=1/2/3/4$ and conduct corresponding ablation study. Evaluation results are shown as Table~\ref{table:ablation_t}. Based on the results, we find that: \textbf{1)} the overall accuracy are robust with different ${k}$ values, and \textbf{2)} introducing prompt ensemble benefits to tail classes (+0.56\% in terms of few-shot accuracy), meanwhile using top-2 best matched prompts for ensemble achieves the best results. Therefore, we choose ${k}=2$ during training and testing.  
We also examine the impact of the ensemble token number $k$ during phase 2. Intuitively, introducing $k$ can enhance accuracy for tail classes by leveraging more class-specific knowledge for recognition. Thus, we explore $k = 1/2/3/4$ and conduct a corresponding ablation study. The evaluation results are presented in Table~\ref{table:ablation_t}.
From our findings, we observe two key points: \textbf{1)} The overall accuracy remains consistent across different $k$ values, indicating robust performance, and \textbf{2)} Introducing prompt ensemble benefits tail classes, contributing to a notable increase in few-shot accuracy (+2.53\%). Moreover, employing the top-2 best matched prompts for ensemble yields the most favorable outcomes.
Consequently, we select $k = 2$ for both training and testing phases based on these results.

\subsection{Effect of Dual Sampling in Phase 2}\label{sec:ablation_dualsample}
% To evaluate the effect of dual sampling in phase 2, we conduct a series of experiments, which is shown as Table~\ref{table:ablation_dual_sampling}. Compared to type (a), type (b) achieves $\sim$0.2\% accuracy improvement in terms of overall accuracy, meanwhile surpasses 1.6\% improvement in terms of many-shot accuracy. These results indicate that: introducing dual sampling strategy with proper $\gamma$ can lead to better overall performance and reduce the overfitting from balanced sampling only, but dual sampling with too large weight may lead to negative effect on overall accuracy. 
To assess the impact of dual sampling in phase 2, we conducted a series of experiments detailed in Table~\ref{table:ablation_dual_sampling}. In comparison to type (a), type (b) demonstrates approximately a 0.6\% increase in overall accuracy and surpasses a 0.2\% improvement in many-shot accuracy. These findings suggest that introducing a dual sampling strategy with an appropriate $\gamma$ can enhance overall performance and mitigate overfitting that may occur with balanced sampling alone. However, employing dual sampling with excessively large weights may potentially reduce overall accuracy, highlighting the importance of parameter tuning in this strategy.

\subsection{Effect of Asymmetric GCL Loss}
% To evaluate the effect of adding asymmetric gradient re-weighting design into GCL loss, we conduct ablation study between $\mathcal{L}_{\text{A-GCL}}$ and standard GCL loss~\cite{Li2022Long}. Without loss of generality, we conduct both experiments on phase 2. The quantitative results are shown as Table~\ref{table:asym_gcl}, LPT with $\mathcal{L}_{\text{A-GCL}}$ surpasses the counterpart with GCL loss by 0.49\% and 1.03\% in terms of overall accuracy and few-shot accuracy. These results further demonstrate the effect of $\mathcal{L}_{\text{A-GCL}}$.
To evaluate the impact of incorporating asymmetric gradient re-weighting into the GCL loss function, we conducted an ablation study comparing $\mathcal{L}_{\text{A-GCL}}$ against the standard GCL loss as described by Li \emph{et al.}~\cite{Li2022Long}. Both experiments were conducted during phase 2 for comprehensive evaluation. The quantitative results are presented in Table~\ref{table:asym_gcl}, revealing that LPT++(V) with $\mathcal{L}_{\text{A-GCL}}$ outperforms its counterpart using the GCL loss by 0.92\% in overall accuracy and by 3.65\% in few-shot accuracy. These findings underscore the efficacy of $\mathcal{L}_{\text{A-GCL}}$ in improving model performance.
